# Supplementary material for: BagPipe: Accelerating Deep Recommendation Model Training
Source: arXiv:2202.12429 source file (2023-11-01)
Supplement: Supplementary file 1 [file appendix.tex]

\section{Appendix}

\subsection{Additional Discussion}
Here we discuss some more features of \system.

\noindent\textbf{Transparency to the user.} Unlike prior work~\cite{yin2021ttrec, adnan2021high} \system is completely transparent to the user. It produces the exact same result which a user would have got if they ran vanilla synchronous training. Our prefetching and caching guarantees are similar in spirit to out of order executions performed in computer architecture~\cite{hwu1986hpsm}.\\

\noindent\textbf{Memory pressure.} Since \system stores the local embedding caches in the accelerator memory it can lead to extra memory pressure on accelerator memory. However, we observe that the memory requirement of dense NN parameters is quite small, \ie at batch size of 2048 dense NN parameters only consumed 1.8 GB of accelerator memory out of the 16 GB available on a V100 memory. This leaves ample space for caching embeddings. We also allow users to configure a maximum cache size and adaptively adjust the lookahead values to make sure the cache size remains bounded. (Section~\ref{sec:bpipe_config})
If in future the memory requirements of dense NN drastically increase, we can investigating moving a portion of cache to CPU memory.\\

\noindent\textbf{Performance on slow networks.} If embedding fetch is extremely slow (say due to a slow network connection), \system can not guarantee that embedding fetch for a batch from the remote embedding server will complete before the training begins. Hence it will have to block. This is because \system relies on overlapping embedding fetch with computation of dense parameters. However, if the fetch is slower than compute we will start observing the latency of embedding fetch in the train loop.  In the data-center setting we observe that \system is able to completely overlap the training time with embedding fetch and hides the fetch latency. However,  even in the case embedding fetch is slow, \system is expected to perform significantly better than baseline because of overall reduction in number of embedding fetches due to caching.

% \section{Timeline for recommendation training}
% In this section we show \system is capable to overlap almost all the operations concerning with regards to embedding access and write back. We study this with the aid of timelines. 

\subsection{Effect of \lkval of Cache churn}
Next we look at the cache churn as a function of \lkval. We define cache churn as the amount of data read and evicted from the cache during one epoch. In Figure~\ref{fig:effect_of_lookahead_cache_churn} we observe that as \lkval increases, the amount of cache churn decreases, and thus, the network traffic generated by cache evictions or additions will decrease. We do note that the cache churn decreases sub-linearly with linear increase in \lkval. This is because in \system we pre-fetch a number of cold embeddings which are used only for one iteration, therefore increasing \lkval does not decrease the amount of cache churn linearly.

\begin{figure}
    \includegraphics[width=0.9\linewidth]{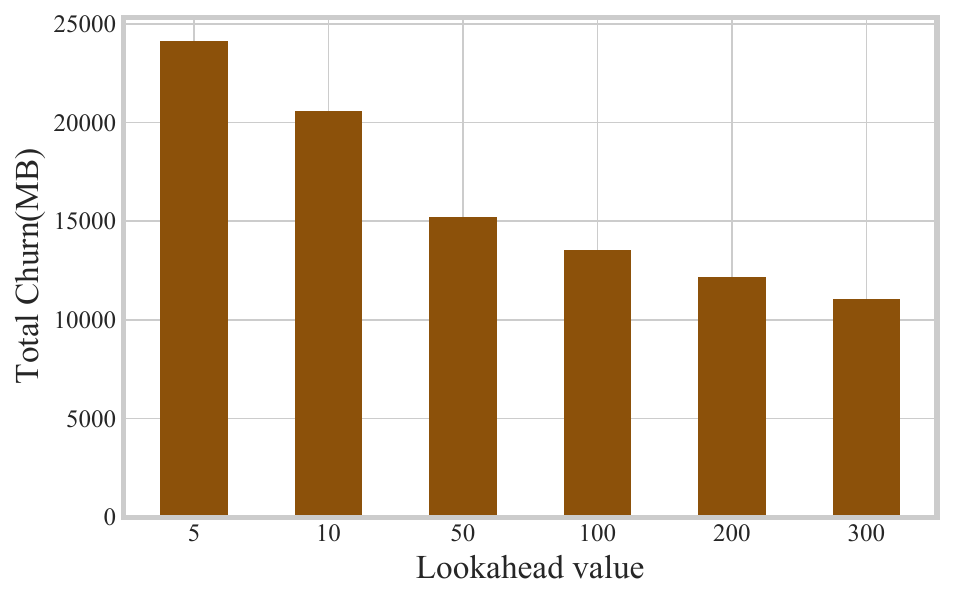}
    \vspace{-0.2in}
    \caption{\small{\textbf{Cache churn in \system as we vary \lkval}}}
    \label{fig:effect_of_lookahead_cache_churn}
\end{figure}

\begin{figure*}[t]
    \includegraphics[width=0.9\linewidth]{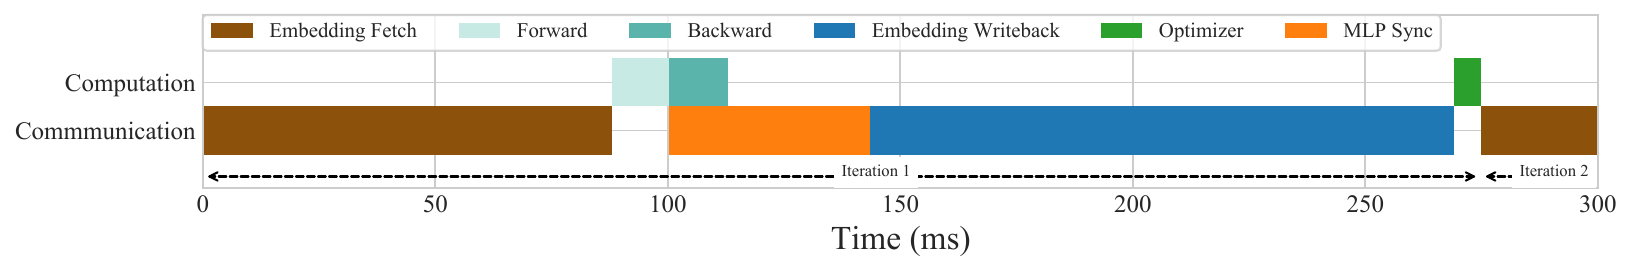}
    \centering
    \vspace{-0.1in}
    \caption{\small{\textbf{Timeline of Operations performed by DLRM-Base for first 300ms}: The above figure shows the various operations performed by DLRM-Base over the course of two iterations. We observe that DLRM baseline can only overlap the synchronization of MLP parameters with the backward pass. Rest of the operations are performed on the critical training path. Only around 8\% of time per iteration is spent on compute.}}
    \label{fig:dlrm_timelint}
    
\end{figure*}

\begin{figure*}[t]
    \includegraphics[width=0.9\linewidth]{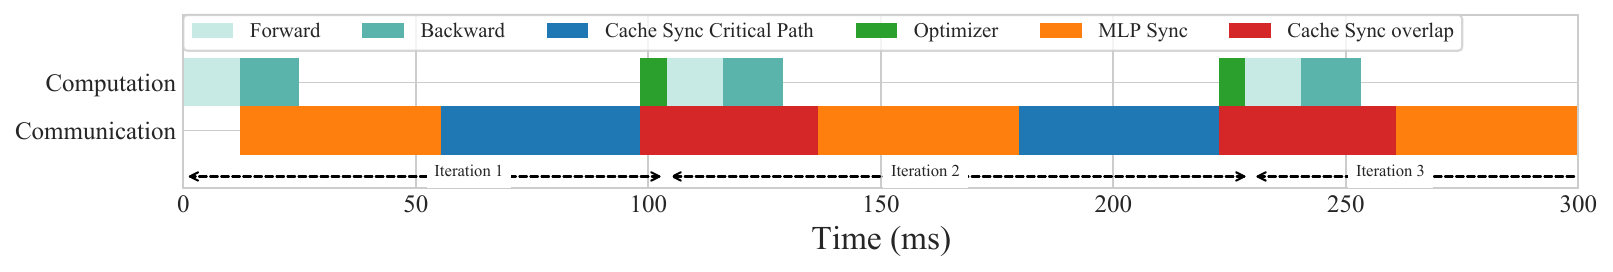}
    \centering
    \vspace{-0.1in}
    \caption{\small{\textbf{Timeline of Operations performed by \system for first 300ms}: The above figure shows the timeline of operations performed by \system for DLRM model. We show that \system has the potential to almost overlap large portions of communication with compute. However, since the compute performed by DLRM is only ~30ms, we still see some portion of communication on the critical path. Further compared to DLRM baseline in Figure~\ref{fig:dlrm_timelint} we also don't have any embedding fetch operations in our critical path as they are handled by our dynamic cache and embedding prefetch. }}
    \label{fig:bagpipe_timeline}
    \end{figure*}
    
\begin{figure*}[t]
    \centering
    \includegraphics[width=0.9\linewidth]{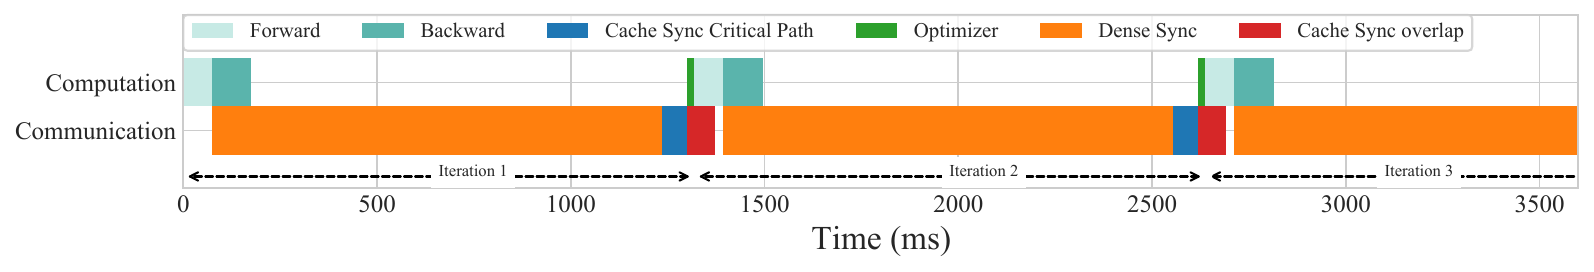}
     \caption{\small{\textbf{Timeline of Operations performed by \system with FGCNN model for first 3600ms}: The above figure shows the timeline of operations performed by \system on FGCNN model. We show that unlike in case of \system with DLRM model, here \system is able to overlap non-critical cache synchronization with the forward pass. This is because FGCNN is a large model which leads to high forward and times.}}
    \label{fig:bagpipe_fgcnn_timeline}
\end{figure*}

\subsection{Effect of \system on critical path of training}
\label{sec:apdx_timelines}
We study the effect of \system's optimizations by plotting a timeline of operations performed by Facebook's DLRM-Base implementation and comparing it with \system's timeline. In Figure~\ref{fig:dlrm_timelint} we show the timeline of operations performed by Facebook's DLRM-Base implementation while training the DLRM model on Criteo Kaggle.  We observe that within an iteration 212ms are spent in embedding fetch and embedding writeback by Facebook's DLRM-Base. 
In Figure~\ref{fig:bagpipe_timeline} we show \system's timeline for training and we observe that \system just spends 43ms per iteration on embedding related operation. To make our comparison fair, we have excluded the data loading time in these figures and only focus on the computation and communication threads.  

%  to Pytorch DLRM-Base w

\subsection{Overlapping Embedding synchronization}
In Section~\ref{sec:bagpipe_overlap} we discussed how \system can overlap a significant portion of cache synchronization with the forward and backward pass. In Figure~\ref{fig:split_diff} we also showed that for DLRM model \system in not able to reach the lower bound of the communication on the critical path. We study why \system is not being able to reach lower bound with the aid of timelines.
In Figure~\ref{fig:bagpipe_timeline} we observe that the time required for synchronization is significantly more than the forward pass. Due to this a significant portion of cache synchronization spills over onto the critical path. In Figure~\ref{fig:bagpipe_fgcnn_timeline} we observe that time required for cache synchronization is almost equal to the time for forward pass. Therefore, in case of FGCNN we are able to completely overlap the synchronization of emebeddings which are not needed in the next iteration. These timelines show that if the recommendation model has a large forward compute time then \system is capable of overlapping synchronization of embeddings that are not required in the next iteration.
%entries that are .  

% \begin{figure*}
%     \centering
%     \includegraphics[width=0.9\linewidth]{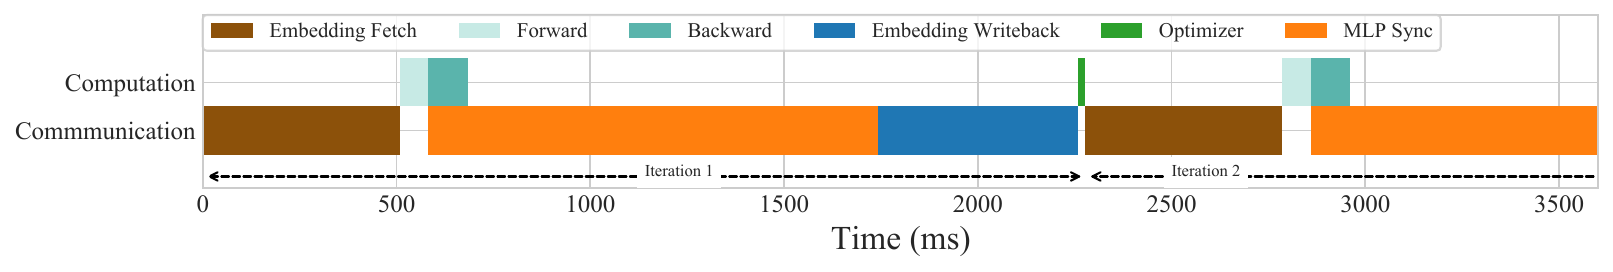}
%      \caption{\small{\textbf{Timeline of Operations performed by \system for first 3600ms in \system no cache no prefetch}: The above figure shows the timeline of operations performed by \system. We show that \system has the potential to almost overlap large portions of communication with compute. However, since the compute performed by DLRM is only ~30ms, we still see some portion of communication on the critical path. Further compared to DLRM baseline in Figure~\ref{fig:dlrm_timelint} we also don't have any embedding fetch operations in our critical path as they are handled by our dynamic cache and embedding prefetch. }}
%     \label{fig:bagpipe_fgcnn_overlap_timeline}
% \end{figure*}

%  In Figure~\ref{fig:effect_of_lookahead_cache_churn} we observe that as look-ahead value is increased the churn decreases and thus, the network traffic generated by cache evictions or additions will decrease.  
